# Supplementary material for: Direct Observation of Coherent Longitudinal and Shear Acoustic Phonons in TaAs Using Ultrafast X-ray Diffraction
Source: arXiv:2011.07196 source file (2022-02-28)
Supplement: Supplementary file 1 [file supplemental_materials.pdf]

# Supplemental Material for
# Direct Observation of Coherent Longitudinal and Shear Acoustic Phonons in TaAs Using Ultrafast X-ray Diffraction

## CONTENTS


I. Ultrafast Dynamics of the (103) Bragg Peak 2

II. Truncation Rod Scattering: Rotation Scans 2

III. Calculated Phonon Polarization 3

IV. Calculated Phonon Dispersion 4

V. Spectral Lineshape Asymmetry of the Longitudinal Acoustic Phonon Mode 5

VI. Numerical simulations with a Two-Temperature Model 7

VII. Optically-Induced Lattice Modulations in an Anisotropic Medium 7

VIII. Truncation Rod Scattering: Acoustic Waves 11

IX. Modeling the Electronic Structure of Dynamically Strained TaAs 13

References 14

## I. ULTRAFAST DYNAMICS OF THE (103) BRAGG PEAK

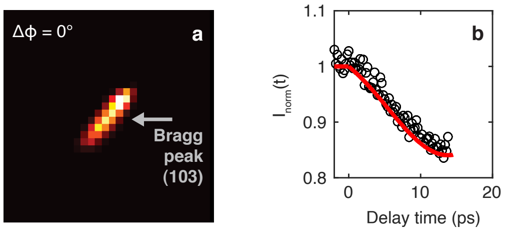


FIG. S1. (a) Two-dimensional XRD images, showing the Bragg peak (103) in equilibrium without optical pumping, and (b) the time-resolved XRD signal at the (103) peak.

We also observed time-resolved diffraction signals at the Bragg peak (103), as shown in Fig. S1. The non-equilibrium dynamics at the Bragg peak can be described by a time-dependent Debye-Waller (DW) model, indicating the time scale for energy transfer to the lattice via redistribution of photoexcited carriers [1]. We fit the data using the function $I(t) = I_0(1 - e^{-t/\tau_\mathrm{B}})$, revealing that energy is transferred from photoexcited carriers to the lattice within $\tau_\mathrm{B} \sim 10$ ps in TaAs. This is comparable to the relaxation time scales of $< 2$ ps for carrier cooling after optical excitation in TaAs; the lifetime measured by optical pump-probe spectroscopy can be shorter, since carriers can incoherently couple to many phonon modes [2].

## II. TRUNCATION ROD SCATTERING: ROTATION SCANS

Consider elastic X-ray scattering under the phase matched condition for truncation rod scattering (TRS):

$$\vec{k'} = \vec{k} + \vec{G} + q\hat{n} = \vec{k} + \vec{Q} \tag{1}$$

$$\vec{k} = k\left(\cos\alpha\cos\phi, \cos\alpha\sin\phi, -\sin\alpha\right) \tag{2}$$

$$\vec{G_{hkl}} = G\left(\cos\theta_1, \cos\theta_2, \cos\theta_3\right) \tag{3}$$

Here we use crystal coordinates defined such that a general vector can be described as $\vec{v} = (\vec{v}\cdot\hat{t_1})\hat{t_1} + (\vec{v}\cdot\hat{t_2})\hat{t_2} + (\vec{v}\cdot\hat{t_3})\hat{t_3} = (\vec{v_1}, \vec{v_2}, \vec{v_3})$, with orthonormal vectors $\hat{t_i}$, as shown in Fig. 1 of the main text. We choose the surface normal vector to be the third component, such that $\hat{t_3} = \hat{n}$. Furthermore, we define directional cosines for the reciprocal lattice vector with respect to our coordinate system as $\cos\theta_i = \hat{G}\cdot\hat{t_i}$. We will use parentheses without commas to denote $k$-space vectors in terms of the reciprocal lattice, i.e. $\vec{K} = (\eta\kappa\xi) = \eta\vec{b_1} + \kappa\vec{b_2} + \xi\vec{b_3}$, where $\vec{b_1} = 2\pi/a\hat{k_x}$, $\vec{b_2} = 2\pi/a\hat{k_y}$, and $\vec{b_3} = 2\pi/c\hat{k_z}$ are reciprocal vectors under a tetragonal convention (TET), as is defined by the $I4_1$md space group of TaAs. When $\eta = h, \kappa = k, \xi = l$ are all integers, this corresponds to a reciprocal lattice vector $\vec{G}_{hkl}$. For a grazing angle, $\alpha > 0$, a symmetric Bragg peak is defined as $\theta_1 = \theta_2 = \pi/2, \alpha_{symm} = \theta_B$. $\phi$ denotes a rotation angle about the surface normal, $\hat{n}$, that the X-ray beam makes with respect to some fixed direction, $\hat{t_1}$, of the crystal surface.

From Eq. (1-3), we can derive the following equation

$$-2\vec{k}\cdot\vec{Q} = Q^2 = G^2\left(\cos\theta_1^2 + \cos\theta_2^2 + (\cos\theta_3 + q/G)^2\right) \tag{4}$$

$$= -2\vec{k}G\left(\cos\alpha(\cos\phi\cos\theta_1 + \sin\phi\cos\theta_2) - \sin\alpha(\cos\theta_3 + q/G)\right) \tag{5}$$

This can be rewritten as

$$\cos\theta_1\cos\phi + \cos\theta_2\sin\phi = \tan\alpha(\cos\theta_3 + q/G) - \frac{Q^2}{2kG\cos\alpha}, \tag{6}$$

which gives

$$\phi(q) = \cos^{-1}\left(\pm\frac{\sin\alpha(\cos\theta_3 + q/G) + Q^2/2Gk}{\cos\alpha\sqrt{\cos^2(\theta_1) + \cos^2(\theta_2)}}\right) + \tan^{-1}\left(\frac{\cos\theta_2}{\cos\theta_1}\right), \tag{7}$$

where we have made use of the identity

$$A\cos\phi + B\sin\phi = C\cos\left(\phi + \tan^{-1}\left(-B/A\right)\right) \tag{8}$$

$$A = \cos\theta_1, \tag{9}$$

$$B = \cos\theta_2, \tag{10}$$

$$C = \sqrt{\cos^2\theta_1 + \cos^2\theta_2}, \tag{11}$$

where the positive (negative) sign corresponds to $A = \cos\theta_1 > (<)0$.

Thus, for $q = 0$ and $\cos\theta_3 \neq 1$ we find the asymmetric Bragg condition,

$$\phi_0 = \phi(q=0) = \cos^{-1}\left(\frac{\sin\alpha\cos\theta_3 - \lambda/2d}{\mathrm{sgn}(\cos\alpha\sqrt{\cos\theta_1{}^2 + \cos\theta_2{}^2})}\right) + \tan\left(\frac{\cos\theta_2}{\cos\theta_1}\right)^{-1} \tag{12}$$

where we use $G/2k = \lambda/2d$ and $Q \approx G$, for $\lambda$ denoting the X-ray wavelength, while $d$ defines the distance between Bragg planes. Alternatively, from Eq. (1) and Eq. (2) we get,

$$q^2 + 2bq + c = 0 \tag{13}$$

$$b = G\cos\theta_3 - k\sin\alpha \tag{14}$$

$$c = G^2 + 2\vec{k}\cdot\vec{G} \tag{15}$$

$$q = -b \pm \sqrt{b^2 - c} \tag{16}$$

where $\vec{k}\cdot\vec{G} = kG\left(\cos\alpha(\cos\phi\cos\theta_1 + \sin\phi\cos\theta_2) - \sin\alpha\cos\theta_3\right)$. Near the Bragg peak, $q \ll 2b$, and $c = (\vec{G}+\vec{k})^2 - k^2 \ll b$, allowing us to take $\Delta\phi = \phi - \phi_0 \ll 1$, such that a linear relation for small $q$ can be obtained by considering a first order expansion in $\phi$,

$$q \approx \Delta\phi G k \cos\alpha \frac{\sin\phi_0\cos\theta_1 - \cos\phi_0\cos\theta_2}{G\cos\theta_3 - k\sin\alpha} \tag{17}$$

In TaAs, we measured TRS from the $\vec{G} = (103)$ Bragg peak to the surface normal $\vec{n} = (112)$. TaAs has a tetragonal lattice, with $a = 3.4348$ Å and $c = 11.641$ Å. We take the X-ray photon energy $E = 9518$ eV ($\lambda = 1.3026$ Å$^{-1}$), the incident angle $\alpha = 3°$, and the rotation angle $\phi = 74.1°$ for the (103) Bragg peak. We measured truncation rod scattering along the $(103) - \xi(112)$ direction by varying the rotation angle, with $\Delta\phi = -0.15°, -0.3°$, and $-0.5°$, in which a phonon momentum, $q$, corresponding to $\xi = 0.0153$ is given for $\Delta\phi = -0.5°$.

## III. CALCULATED PHONON POLARIZATION

Elastic waves in crystals follow the equation of motion [3]:

$$\rho\frac{\partial^2 u_i}{\partial t^2} = C_{iklm}\frac{\partial^2 u_m}{\partial x_k \partial x_l} \tag{18}$$

with an elastic modulus tensor $C_{iklm}$, a displacement vector $u_i = x_i' - x_i$ (where $x_i'$ is the displaced point and $x_i$ is the point before displacement), and a mass density $\rho$. Considering a monochromatic elastic wave in the form of $u_i = u_0\exp(j(\mathbf{k}\cdot\mathbf{r} - \omega t))$, where $u_i = \delta_{im}u_m$, then we can write Eq. (18) as:

$$(\rho\omega^2\delta_{im} - C_{iklm}k_k k_l)u_m = 0 \tag{19}$$

For TaAs, values for the elastic tensor elements, $C_{iklm}$, can be obtained from previous calculations [4], and are shown in Table I.

From Eq. (19), the $C_{iklm}k_k k_l$ term can be written in matrix form:

$$C_{iklm}k_l k_m = \begin{bmatrix} C_{11}k_x^2 + C_{66}k_y^2 + C_{44}k_z^2 & (C_{12}+C_{66})k_x k_y & (C_{13}+C_{44})k_x k_z \\ (C_{12}+C_{66})k_x k_y & C_{66}k_x^2 + C_{11}k_y^2 + C_{44}k_z^2 & (C_{13}+C_{44})k_y k_z \\ (C_{13}+C_{44})k_x k_z & (C_{13}+C_{44})k_y k_z & C_{44}k_x^2 + C_{44}k_y^2 + C_{33}k_z^2 \end{bmatrix} \tag{20}$$

TABLE I. Elastic modulus tensor of TaAs

| $C_{ab}$ (GPa) | $C_{iklm}$ |
|---|---|
| $C_{11} = 310.5$ | $C_{xxxx} = C_{yyyy}$ |
| $C_{12} = 164.2$ | $C_{xxyy} = C_{yyxx}$ |
| $C_{13} = 128.9$ | $C_{xxzz} = C_{zzxx} = C_{yyzz} = C_{zzyy}$ |
| $C_{33} = 256.1$ | $C_{zzzz}$ |
| $C_{44} = 94.5$ | $C_{xzxz} = C_{yzyz} = C_{xzzx} = C_{yzzy} = C_{zxxz} = C_{zyyz}$ |
| $C_{66} = 194.5$ | $C_{xyxy} = C_{yxyx} = C_{yxxy} = C_{xyyx}$ |

where a non-zero solution exists only if the determinant of the coefficient is zero, i.e. $|C_{iklm}k_lk_m - \rho\omega^2\delta_{im}| = 0$. By using the experimental geometric conditions for X-ray truncation rod scattering with $\vec{k} = (112)$ and $\rho = 12.4g/cm^3$, we find phonon polarization vectors:

$$\vec{v}_{\mathrm{TA1}} = 0.71\hat{k}_x - 0.71\hat{k}_y \tag{21}$$

$$\vec{v}_{\mathrm{TA2}} = 0.19\hat{k}_x + 0.19\hat{k}_y - 0.96\hat{k}_z \tag{22}$$

$$\vec{v}_{\mathrm{LA}} = 0.68\hat{k}_x + 0.68\hat{k}_y + 0.26\hat{k}_z \tag{23}$$

where TA and LA denote the transverse and longitudinal acoustic phonon modes, respectively. We display the TA2 and LA modes in Fig. 3(c), along with the quasi-shear (QS) and quasi-longitudinal (QL) modes observed from our TRS data. The angle between the QL polarization $\vec{v}_{\mathrm{LA}}$ and the surface normal vector $\vec{n} = (112)$ is 7.52°.

We also notice a close relation between the QS mode and shift current, which has recently been observed in terahertz emission and time-resolved second harmonic generation experiments [5, 6]. From Fig. 3(a) of the main text, we find that both the QS phonon polarization and shift current are nearly parallel to one another, with each being directed slightly off the $(11\bar{1})$ axis. This suggests that the shift current might contribute to the generation of the QS mode in TaAs via an inverse piezoelectric process [7], resulting in comparable amplitudes for the QS and QL modes; this is unusual, considering the typical thermoelastic process for acoustic strain generation [8].

## IV. CALCULATED PHONON DISPERSION

We performed first principles calculations of the phonon dispersion to compare with our experimental results. The phonon momentum $q$ is parallel to the (112) surface normal. As shown in Fig. S2, the (112) vector spans from zone center ($\Gamma$) of the first Brillouin zone (BZ) to the $\Gamma$ point of the neighboring zone. An arbitrary point along this line can be expressed as $\xi(112)$, such that $\xi = 0$ corresponds to the $\Gamma$ point in the first BZ, while $\xi = 1$ denotes the $\Gamma$ point

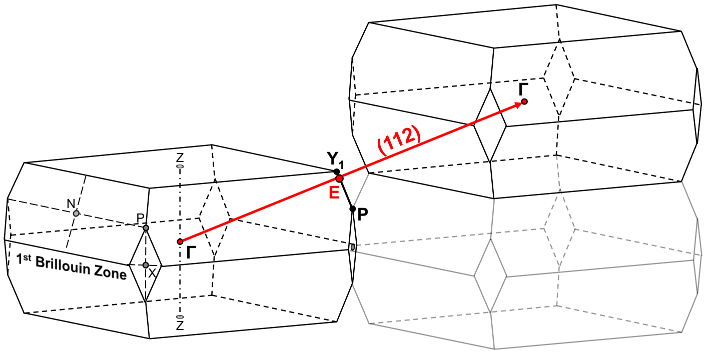


FIG. S2. Brillouin zones of body centered tetragonal lattice type 2 (BCT2).

in the neighboring BZ. Note that $(112) = 1 \times \vec{b_1} + 1 \times \vec{b_2} + 2 \times \vec{b_3}$, where $\vec{b_1} = 2\pi/a\hat{k_x}$, $\vec{b_2} = 2\pi/a\hat{k_y}$, and $\vec{b_3} = 2\pi/c\hat{k_z}$ are primitive vectors under the TET convention defined earlier.

To extract the phonon dispersion along the (112) direction, we must determine the $k$-space point (labelled with E) where the (112) line crosses the first Brillouin zone boundary. Due to symmetry, this point should be on the line between the high symmetry points of $Y_1$ and P:

$$Y_1 = \frac{1}{2}\vec{b_1'} + \frac{1}{2}\vec{b_2'} - \frac{a^2}{2c^2}\vec{b_3'} \tag{24}$$

$$P = \frac{1}{4}\vec{b_1'} + \frac{1}{4}\vec{b_2'} - \frac{1}{4}\vec{b_3'} \tag{25}$$

where $\vec{b_i'}$'s are primitive reciprocal lattice vectors in a type 2 body-centered tetragonal lattice(BCT2):

$$\vec{b_1'} = \vec{b_3} + \vec{b_1}, \vec{b_2'} = \vec{b_2} + \vec{b_3}, \vec{b_3'} = \vec{b_1} + \vec{b_2} \tag{26}$$

Using these conditions, we can express the $Y_1$ and P points with $\vec{b_i}$ under the TET convention:

$$Y_1 = \left(\frac{1}{2}\left(1 - \frac{a^2}{c^2}\right), \frac{1}{2}\left(1 - \frac{a^2}{c^2}\right), 1\right) \tag{27}$$

$$P = \left(\frac{1}{2}, \frac{1}{2}, \frac{1}{2}\right) \tag{28}$$

Thus, we find that $\xi = 0.4633$ for E $= \xi(112)$, given E to be the intersection between the (112) vector and $\overline{Y_1 P}$.

We extracted the phonon dispersion along the line from Γ to E as shown in Fig. 3(b,c) in the main text. Here, we plot the phonon frequency as a function of $\xi$, finding it to be linear in the phonon momentum $q\hat{n} = -\xi(112)$, giving $\vec{Q} = \vec{G} + q\hat{n} = (103) - \xi(112)$. For $\xi = 1$, $\vec{Q} = (0\bar{1}1)$, which corresponds to a $q = 2.803$Å. The quasi-longitudinal (QL) and the quasi-shear (QS) modes are respectively indicated by orange circles and blue diamonds (Fig. 3(c)), which closely match the calculated acoustic phonon dispersion.

The phonon frequencies were determined using first-principles methods implemented in the plane wave density functional theory (DFT) package QUANTUM ESPRESSO (QE) [9]. Ground state electronic wave functions were calculated using a 12×12×12 Monkhorst-Pack k-point grid and an energy cut-off of 60 Ry, and lattice and atomic positions were relaxed to a force threshold of $10^{-6}$ Ry/aB. The Perdew-Burke-Ernzerhof (PBE) generalized gradient approximation (GGA) was used for the exchange correlation functional, and fully-relativistic pseudopotentials were generated using the Optimized Norm-Conserving Vanderbilt PSeudoPotential (ONCVPSP) code [10] in order to account for spin-orbit coupling (SOC). Density functional perturbation theory (DFPT) was applied to the ground state information using the PHONON [11–13] code included in QE, and a commensurate 4×4×4 q-point grid was used to calculate the phonon dispersion.

A comparison between first principles calculations and the experimentally determined acoustic phonon dispersion along the (112) direction near the Brillouin zone center is shown in Fig. 3(b,c) as a function of phonon momentum $q$ (defined in Eq. (1)). Here, the calculated dispersion (Fig. 3(b)) reveals three acoustic branches that are attributed to a single longitudinal acoustic (LA) mode and two transverse acoustic (TA) modes. This agrees well with the experimentally determined $q$-dependence of the QL and QS modes obtained from our tr-XRD measurements, as shown in Fig. 3(c) with solid lines.

We simulated the phonon dispersion by using elastic modulus tensor calculations (dashed lines in Fig. 3(c)), which shows agreement with the phonon dispersion from first principles calculations (solid lines in Fig. 3(c)), allowing us to conclude that the observed QL and QS modes are the LA and TA2 modes, respectively, in TaAs.

We note that the phonon dispersion obtained from first principles calculations are for polarization modes exactly along, or perpendicular to, the propagating wavevector, (112). This might be the reason for the discrepancy between the experimental data and the simulated phonon dispersion in Fig. 3(c).

## V. SPECTRAL LINESHAPE ASYMMETRY OF THE LONGITUDINAL ACOUSTIC PHONON MODE

Time-domain data for the QL mode likewise supports the observation of a positive frequency chirp in the dynamics. As shown in Fig. S3, little difference is seen between the chirped and un-chirped models at early time delays (Fig.

S3(a)), but longer time delays at $t > 40$ ps reveal the chirped model to show better agreement with the raw data (Fig. S3(b)).

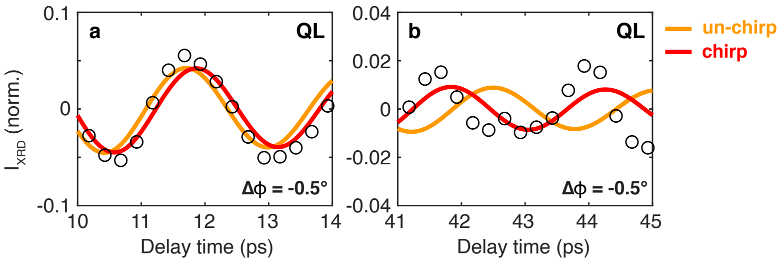


FIG. S3. The raw data of the QL mode for $\Delta\phi = -0.5°$ in the time-domain from (c) 10-14 ps and (d) 41-45 ps, where orange and red solid lines are fit results for the un-chirp and chirp models, respectively.

We plot Fourier transforms of the oscillatory signals for $\Delta\phi = -0.5°$ over various time windows, as shown in Fig. S4. For a fixed end point of 40 ps, the time window shrinks with increasing delay, leading to a diminished low-frequency component in the longitudinal mode ($\sim$400 GHz) while keeping its asymmetric spectral lineshape, which is not the case for the shear mode at $\sim$200 GHz.

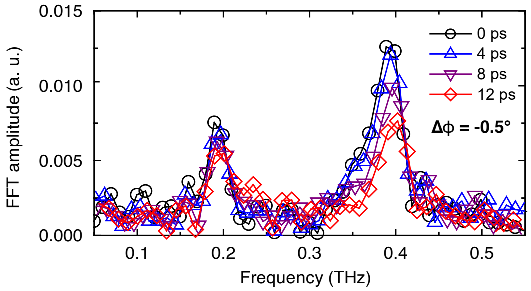


FIG. S4. Fourier transforms of oscillatory signals over different time windows, starting at 0 ps (black), 4 ps (blue), 8 ps (purple), and 12 ps (red) and all extending to 40 ps.

To simulate the asymmetric lineshape of the QL mode for $\Delta\phi = -0.15°$ and $-0.3°$, we used a model considering a time-varying increase in the phonon frequency, as described in the main text: $I_{osc}(t) = A\cos(2\pi f(t)t - \varphi)$, where $f(t) = f_0(1 + Ct)$ for a frequency increasing monotonically with time. The time-varying frequency model fits better to the phonon spectra than an un-chirped model for all angles, as shown in Fig. S5, demonstrating that this effect is independent of phonon momentum.

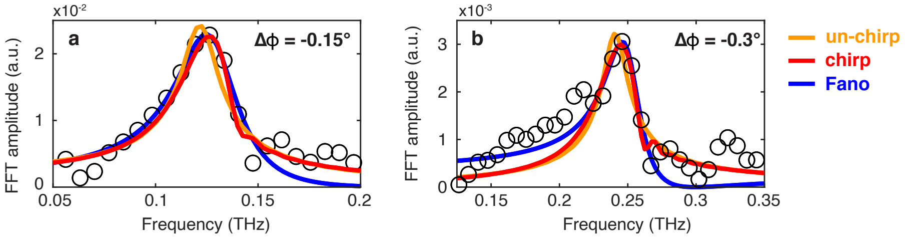


FIG. S5. Fits (solid lines) to the spectral lineshape of the QL mode (open circles) for (a) $\Delta\phi = -0.15°$ and (b) $-0.3°$.

Microscopically, such a positive frequency chirp has been observed using picosecond ultrasonics, in which a broadband strain pulse, injected by impulsive optical excitation, spreads in both time and space through phonon dispersion, but does not produce an asymmetric lineshape [14, 15]. This is unlikely to be due to a nonlinear process, as the overall magnitude of the acoustic strain is small ($<$ 20 pm), and a previous study revealed a negative frequency chirp under strong optical pumping [16], much higher than in our experiments. Instead, the positive chirp and asymmetric

lineshape of the QL mode can be linked to the ambipolar diffusion of photoinduced carriers [17], as we discuss in the main text.

## VI. NUMERICAL SIMULATIONS WITH A TWO-TEMPERATURE MODEL

We simulated electron and lattice temperature dynamics using a two-temperature model, taking carrier diffusion into account [18]. We used various values for the ambipolar diffusivity ($D_e$) of TaAs, which has not been measured before. This reveals a significant heat gradient over an approximate depth ($a$ >100 nm) far greater than the optical skin depth (22 nm) along the surface normal (Fig. S6). Our simulation also shows a rapid thermalization of the lattice after optical excitation, as the electronic and lattice temperatures equilibrate within ∼5 ps, while cooling occurs over a relatively slow (> 100 ps) timescale. This indicates that the rapid development of the thermal gradient is governed by the ambipolar diffusion of photoinduced carriers [17].

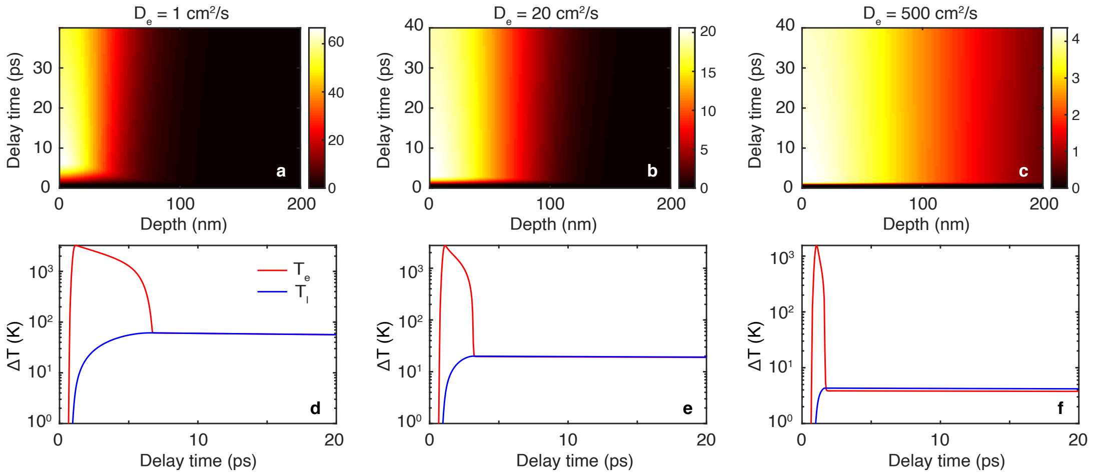


FIG. S6. (a-c) Simulated temporal evolution of lattice heating induced by optical pumping as a function of sample depth and time. (d-f) Time evolution of the electronic ($T_e$) and lattice ($T_l$) temperatures induced by a femtosecond optical pulse. We used ambipolar diffusivity values of $D_e$ = (a,d) 1 cm$^2$/s, (b,e) 20 cm$^2$/s, and (c,f) 500 cm$^2$/s, which all show fast development of a heat gradient within <∼ 5 ps over a depth of ∼ 100 nm.

## VII. OPTICALLY-INDUCED LATTICE MODULATIONS IN AN ANISOTROPIC MEDIUM

Despite the observed asymmetric lineshape, the generation of a QL mode under ultrafast optical excitation is a common phenomenon brought on by thermoelastically driven strain wave propagation [19]. In contrast, the observation of a QS mode necessitates the breaking of axial symmetry, which is readily accomplished by choosing an off-axis crystal orientation (e.g., the (112) face of TaAs) [20]. In this specific crystal geometry, the excitation of a QS mode follows from an asynchronous generation mechanism, in which an in-plane strain arises after the initial optical excitation due to a difference in propagation velocities between the LA and TA modes (Fig. S7). In order to analytically resolve the ultrafast laser excitation of QL and QS strains in TaAs, it is required to solve the coupled Newton's second law, which for continuous media can be written as

$$\rho \frac{\partial^2 u_i}{\partial t^2} = \frac{\partial \sigma_{ij}}{\partial x_j} \tag{29}$$

where $u_i$ denotes the acoustic displacement or polarization vector, $\rho$ the mass density and $\sigma_{ij}$ the stress tensor. We only consider the propagation of plane acoustic waves along the out-of-plane $z$ direction, consequently, all partial derivatives associated with the propagation along $x$ and $y$ can be omitted and only the terms where $j = z$ in Eq. (29) remain

$$\rho \frac{\partial^2 u_i}{\partial t^2} = \frac{\partial \sigma_{iz}}{\partial z}, \tag{30}$$

where $\sigma_{iz}$ are the components of the elastic stress tensor in the coordinate axes $(i = x, y, z)$. The general expression of the stress tensor is given by

$$\sigma_{ij} = c_{ijkl}\varepsilon_{kl} - B_{ij}T, \tag{31}$$

where $c_{ijkl}$ is the elastic modulus tensor, $\varepsilon_{kl} = 1/2(\partial u_k/\partial x_l + \partial u_l/\partial x_k)$ the strain tensor, $B_{ij}$ the thermoelastic tensor that follows $B_{ij} = c_{ijkl}\beta_{kl}$ with $\beta_{kl}$ the thermal dilatation tensor, and $T$ the temperature rise induced by the laser. The right hand term in Eq. (31) denotes the stress source driven by the laser, it comprises the laser-induced thermoelastic stress $-B_{ij}T$, while the left hand term denotes the elastic component. By combining Eq. (29) and Eq. (30), we obtain,

$$\rho\frac{\partial^2 u_i}{\partial t^2} = c_{i3k3}\frac{\partial^2 u_z}{\partial z^2} - c_{i3kl}\beta_{kl}\frac{\partial T}{\partial z}, \tag{32}$$

Note that since the dilatation tensor $\beta_{kl}$ is diagonal in the case of TaAs, this last expression can be simplified further.

Since the experimental coordinate system $(x, y, z)$ does not correspond to the [100], [010], [001] crystallographic directions, which form the conventional $(x^*, y^*, z^*)$ coordinate system for tensorial expressions, it is required to calculate the tensors upon a transformation of the coordinate system $(x^*, y^*, z^*)$ into $(x, y, z)$. The most general transformation matrix, to transform these coordinate systems, have the form

$$[a] = \begin{bmatrix} a_{11} & a_{12} & a_{13} \\ a_{21} & a_{22} & a_{23} \\ a_{31} & a_{32} & a_{33} \end{bmatrix}. \tag{33}$$

The calculation of the elastic tensor $c_{mnop}$ in the coordinate system $(x, y, z)$ is derived after transformation of the elastic tensor $c^*_{ijkl}$ from the generic transformation equation of tensors,

$$c_{mnop} = a_{mi}\, a_{nj}\, a_{ok}\, a_{pl}\, c^*_{ijkl}. \tag{34}$$

The Einstein summation notation is used all along to imply summation over repeated indices. The calculation of each component of the transformed tensor carrying full subscripts is cumbersome. Thus, it is possible to adopt abbreviated subscripts and transform the abbreviated tensor from the following equation,

$$[c] = [M][c^*][M]^t, \tag{35}$$

where $[c^*]$ is the untransformed 6×6 elastic matrix in abbreviated form. As in any tetragonal system, including the

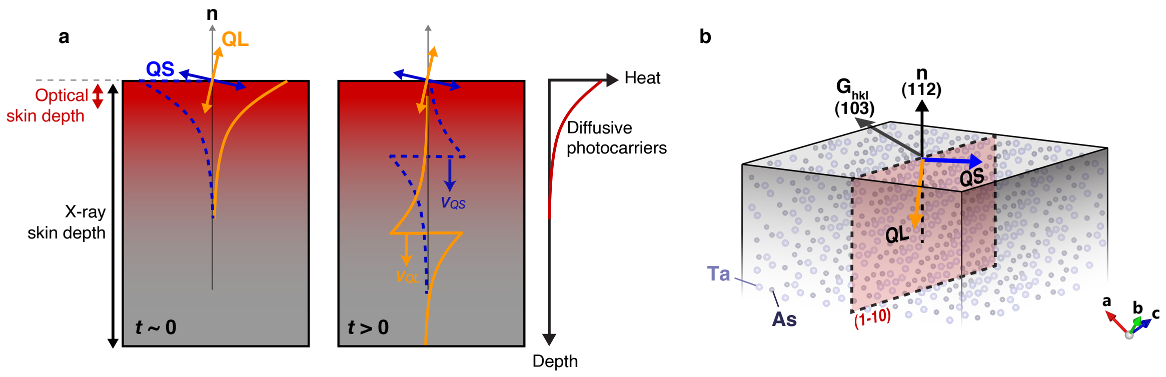


FIG. S7. (a) Schematic showing the laser-excitation of the QL and QS modes. At time $t \sim 0$, the in-plane shear displacements of both modes are perfectly balanced and there is no shear stress or strain until both modes propagate away from the laser-excited area. (b) the polarization of the QL and QS acoustic modes induced by optical pumping in TaAs.

$I4_1md$ space group of TaAs, the elastic tensor contains 6 constants and reads,

$$[c^*] = \begin{bmatrix} c_{11} & c_{12} & c_{13} & 0 & 0 & 0 \\ c_{12} & c_{11} & c_{13} & 0 & 0 & 0 \\ c_{13} & c_{13} & c_{33} & 0 & 0 & 0 \\ 0 & 0 & 0 & c_{44} & 0 & 0 \\ 0 & 0 & 0 & 0 & c_{44} & 0 \\ 0 & 0 & 0 & 0 & 0 & c_{66} \end{bmatrix}. \tag{36}$$

$[M]$ and $[M]^t$ in Eq. (35) are the transformation and transposed transformation matrices, respectively. These matrices can be calculated analytically as in [21],

$$[M] = \begin{bmatrix} a_{11}^2 & a_{12}^2 & a_{13}^2 & 2a_{12}a_{13} & 2a_{13}a_{11} & 2a_{11}a_{12} \\ a_{21}^2 & a_{22}^2 & a_{23}^2 & 2a_{22}a_{23} & 2a_{23}a_{21} & 2a_{21}a_{22} \\ a_{31}^2 & a_{32}^2 & a_{33}^2 & 2a_{32}a_{33} & 2a_{33}a_{31} & 2a_{31}a_{32} \\ a_{21}a_{31} & a_{22}a_{32} & a_{23}a_{33} & a_{22}a_{33}+a_{23}a_{32} & a_{21}a_{33}+a_{23}a_{31} & a_{22}a_{31}+a_{21}a_{32} \\ a_{31}a_{11} & a_{32}a_{12} & a_{33}a_{13} & a_{12}a_{33}+a_{13}a_{32} & a_{13}a_{31}+a_{11}a_{33} & a_{11}a_{32}+a_{12}a_{31} \\ a_{11}a_{21} & a_{12}a_{22} & a_{13}a_{23} & a_{12}a_{23}+a_{13}a_{22} & a_{13}a_{21}+a_{11}a_{23} & a_{11}a_{22}+a_{12}a_{21} \end{bmatrix}. \tag{37}$$

In a very general situation such as in our (112) TaAs sample, the calculation of the elastic tensor has to be performed numerically. Solving Eq. (32) can then be performed analytically and numerically by transposing the results detailed in [20, 22], where the mathematical analysis to solve the thermoelastic laser-excitation in anisotropic media is fully described, to our current model. Shortly, the analytical solutions of the $t$-Fourier transformed surface displacements transmitted in the dielectric medium can be obtained after solving the full set of equations contained in Eq. (32) and taking into account the continuity of the stresses and displacements at the free boundary. The solutions adapted from [20, 22], can be written in the general form,

$$\widetilde{u}_i(z,\omega) = \Gamma_{im}\widehat{T}_{im}(-jk_m,\omega)e^{jk_i z}. \tag{38}$$

where the $\Gamma_{im}$ coefficients expressions are given in [20, 22], $k_i$ are the wavevectors, $\omega$ the angular frequency and $\widehat{T}_{im}$ the $t$-Fourier $x$-Laplace transform of the laser-induced temperature rise. To proceed further, it is required to model the laser-excitation effect itself in order to calculate $\widehat{T}_{im}$. For simplicity, we will assume that the laser-induced temperature rise is instantaneous and we will neglect thermal diffusion which is a rather slow effect as compared to the acoustic excitation process. In this case, the solution of the acoustic displacement amplitudes at the free surface take the simple form,

$$u_i(0,t) = (\frac{F}{\rho c_p})\Gamma_{im}(1 - e^{\alpha v_m t}), \tag{39}$$

where $F = F_0\,(1 - R)$ with $F_0$ the laser fluence and $R$ the sample reflectivity at the pump wavelength, $c_p$ the heat capacity and $v_m$ the elastic velocity of the three different acoustic modes, namely the quasi-longitudinal mode QL and the two quasi-transverse modes $QS_1$ and $QS_2$. The velocity $v_m$ of these modes that are in fact the elastic eigenvectors of the elastic tensor can be calculated from the Christophel equation. Note that at normal incidence, the acoustic reflection of these eigenvectors at the free surface does not lead to acoustic mode conversion, these eigenvectors are preserved upon reflection, which is not the case if the interface is loaded with another material. In this specific case, the reflection coefficients of the quasi-longitudinal mode are [23],

$$R_{qlql} = \frac{(z_l - z_{ql})(z_t + z_{qt}) + \sin^2\alpha(z_t - z_l)(z_{qt} + z_{ql})}{(z_l + z_{ql})(z_t + z_{qt}) + \sin^2\alpha(z_t - z_l)(z_{qt} - z_{ql})}$$
$$R_{qlqt} = \frac{z_{ql}(z_l - z_t)\sin 2\alpha}{(z_l + z_{ql})(z_t + z_{qt}) + \sin^2\alpha(z_t - z_l)(z_{qt} - z_{ql})}$$

where $z_l$, $z_t$, $z_{ql}$, $z_{qt}$ are the acoustic impedances of the two different media, $\alpha$ is the angle between the quasi-longitudinal polarization and the $z$-direction. If the anisotropic medium has a free surface boundary for which $z_l = 0$ and $z_t = 0$, then $R_{qlql} = -1$, $R_{qlqt} = 0$, meaning no conversion of the quasi-longitudinal mode into the quasi-shear

mode can occur. Therefore the excitation of each individual mode can be analyzed independently and from Eq. (39), we can obtain the analytical expression of the vectorial displacements of these modes at the free surface,

$$\begin{aligned} \vec{u}_{QS_1}(0,t) &= (\frac{F}{\rho c_p})(1 - e^{\alpha v_m t})(\Gamma_{11}\,\vec{t_1} + \Gamma_{12}\,\vec{t_2} + \Gamma_{13}\,\vec{t_3}) \\ \vec{u}_{QS_2}(0,t) &= (\frac{F}{\rho c_p})(1 - e^{\alpha v_m t})(\Gamma_{21}\,\vec{t_1} + \Gamma_{22}\,\vec{t_2} + \Gamma_{23}\,\vec{t_3}) \\ \vec{u}_{QL}(0,t) &= (\frac{F}{\rho c_p})(1 - e^{\alpha v_m t})(\Gamma_{31}\,\vec{t_1} + \Gamma_{32}\,\vec{t_2} + \Gamma_{33}\,\vec{t_3}). \end{aligned} \tag{40}$$

The calculation of the $\Gamma_{im}$ coefficients can be performed numerically as in [20, 22] for the quantitative evaluation of the acoustic displacements of the modes. We obtain the value of, at a given laser fluence $F_0$ of 2.86 mJ/cm$^2$ and a sample reflectivity $R$ of 0.85 at 800 nm pump wavelength for a grazing incidence condition,

$$(\frac{F}{\rho c_p})[\Gamma_{im}] = \begin{bmatrix} 0 & 11.2 & -3.2 \\ 0 & 0 & 0 \\ 0 & -1.4 & -25.9 \end{bmatrix} \times 10^{-12} \text{ m}. \tag{41}$$

As expected, since the second line in Eq. (41) is zero, the QS$_2$ mode which is in fact a pure shear mode is not detected for symmetry reasons. The amplitude of the QL mode of about $\sqrt{(-1.4)^2 + (-25.9)^2} = 25.9$ pm is 2.2 times higher than the amplitude of the QS$_1$ mode of $\sqrt{(11.2)^2 + (-3.2)^2} = 11.6$ pm. It is important to understand that the excitation of the QS$_1$ mode does not require any shear stress impulse. Due to the elastic anisotropy, a purely longitudinal stress along the normal of the sample can excite both modes. This is at the origin of the so-called asynchronous shear excitation. In our specific situation, the input thermoelastic stress $B^*_{ij}$ in the conventional coordinate system $(x^*, y^*, z^*)$ is indeed purely longitudinal, with only diagonal terms. From the known values of the thermal dilatation coefficients along the $a$ and $c$ lattice dimensions taken from [24], and the elastic coefficients taken from [4], we calculate

$$[B^*] = \begin{bmatrix} 6.55 & 0 & 0 \\ 0 & 6.55 & 0 \\ 0 & 0 & 6.1634 \end{bmatrix} \times 10^6 \text{ Pa/K}. \tag{42}$$

The thermoelastic stress $B_{ij}$ in the experimental coordinate system $(x, y, z)$ is calculated in its contracted form from the relationship,

$$[B] = [M][B^*], \tag{43}$$

where $[M]$ is the transformation matrix of Eq. (37), where we obtain the numerical value,

$$[B] = \begin{bmatrix} 6.22 & 0 & 0.14 \\ 0 & 6.55 & 0 \\ 0.14 & 0 & 6.49 \end{bmatrix} \times 10^6 \text{ Pa/K}. \tag{44}$$

In the experimental coordinate system $(x, y, z)$, a slight off-diagonal component $B_{13}$= 0.14 Pa/K emerges which, after numerical evaluation, is responsible for only 12% of the amplitude for the quasi-shear excitation. This shear stress directly couples to the shear excitation, however, the predominant part of the excitation of the quasi-modes and in particular of the QS$_1$ comes from the diagonal component $B_{33}$ of the input thermoelastic tensor that is responsible for 88% of the amplitude for the quasi-shear excitation. From this thermoelastic model, this mechanism of quasi-shear excitation is purely elastic. In fact, an out-of-plane stress applied to a canted crystal with broken symmetry, that sustain quasi-modes tilted with respect to the sample surface, gives rise to in-plane acoustic displacements as well. If the off-diagonal stress $B_{13}$ is negligible, these acoustic displacements of the two QL and QS$_1$ are perfectly balanced at time zero but arise due to the acoustic mismatch propagation of the modes at two different acoustic velocities, see Fig. S7 [20].

## VIII. TRUNCATION ROD SCATTERING: ACOUSTIC WAVES

In this section, we introduce how we determined the value of acoustic strain from our tr-XRD data. Assuming that the crystal occupies a half-space $z > 0$, and only considering the contribution of one reciprocal lattice vector $\vec{G}$, the electron density is given by

$$\rho_e(\vec{r}) = \theta(z)e^{-j\vec{G}\cdot\vec{r}}, \tag{45}$$

where $\theta(z)$ is the Heaviside step function. In the presence of an acoustic pulse, this becomes

$$\rho_e(\vec{r}) = \theta(z)e^{-j\vec{G}\cdot(\vec{r}+\vec{u}(\vec{r}))}, \tag{46}$$

where $\vec{u}(\vec{r})$ is the acoustic displacement, as defined in the previous section. Assuming that the displacement is small, $\vec{G}\cdot\vec{u} \ll 1$, we get

$$\rho_e(\vec{r}) = \theta(z)(1 - j\vec{G}\cdot\vec{u}(\vec{r}))e^{-j\vec{G}\cdot\vec{r}}. \tag{47}$$

For an acoustic wave propagating along the surface normal, the acoustic displacement is $\vec{u}(\vec{r}) = \hat{e}u_z(z)$, where $\hat{e}$ is a unit vector denoting the polarization.When the acoustic pulse is far from the surface boundary, $z = 0$, such that the acoustic displacement, $u$, vanishes at the boundary, we get

$$\rho_e(\vec{r}) = \theta(z)e^{-j\vec{G}\cdot\vec{r}} - j\gamma Gu(z)e^{-j\vec{G}\cdot\vec{r}}, \tag{48}$$

where $\gamma$ is the cosine of the angle between $\hat{e}$ and $\vec{G}$.

Let us now calculate the structure factor $F = \int \rho_e(\vec{r})e^{i\vec{k}\cdot\vec{r}}d\vec{r}$. By using the substitution $\vec{k} = \vec{q} + \vec{G}$, where $\vec{q}$ is the momentum of an acoustic phonon, the structure factor can be written as

$$F = \int (\theta(z) - j\gamma Gu(z))e^{jq_z z}dz\delta(q_x)\delta(q_y), \tag{49}$$

where $\delta$ denotes a delta-function in $q_x$ and $q_y$. Thus, the structure factor is non-zero only for $\vec{q}$ directed along z, reducing the calculation to a one-dimensional integral

$$F = \int (\theta(z) - j\gamma Gu(z))e^{jq_z z}dz, \tag{50}$$

where $q = q_z = |\vec{q}|$. We now assume that the strain in the acoustic pulse has a bipolar profile given by

$$\frac{du}{dz} = -\eta_0 sgn(z - vt)e^{-|z-vt|/a}, \tag{51}$$

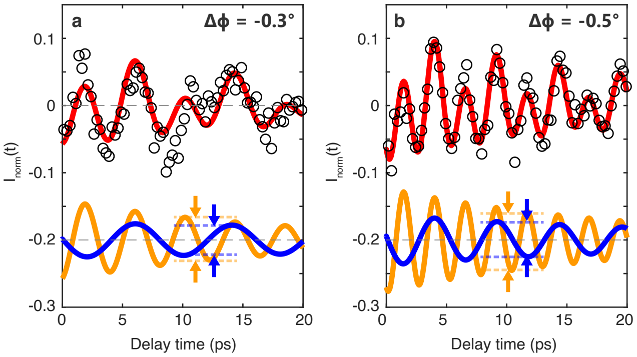


FIG. S8. Time-resolved TRS oscillatory signals from coherent acoustic phonons with (a) $\Delta\phi = -0.3°$ and (b) $-0.5°$. These signals are normalized by the static TRS signal of $S_0 = 1$ at the negative time delay, and we extract the peak-to-peak ratio of the QL (orange) and QS (blue) modes at around $t = 10$ ps to consider cases when the acoustic waves is far from the boundary $z = 0$, as indicated by the dashed lines and solid arrows.

where $v$ is the acoustic velocity, as noted before, $\eta_0$ is the strain amplitude, and $a$ is the acoustic pulse length determined here by the diffusion length of photoinduced carriers ($a \sim 100$ nm). This value can be achieved by ambipolar diffusion with a diffusion length $D_e = \mu k_B T/e$, where $\mu$, $k_B$, $T$, and $e$ are the mobility, Boltzmann constant, temperature, and electron charge, respectively. With $\mu = 3000$ cm$^2$V$^1$s$^{-1}$ at $T = 300$ K [25] and an electron-phonon scattering time of $\tau = 0.62$ ps (revealed by our time-resolved reflectivity change measurements after the 800 nm pump), we obtain $D_e = 77.6$ cm$^2$/s, resulting in a diffusion length of $l = \sqrt{D_e\tau} = 69.4$ nm.

Integrating Eq. (51) then gives a displacement profile of

$$u(z) = \eta_0 a e^{-|z-vt|/a}. \tag{52}$$

Performing the integration in Eq. (50), we obtain

$$F = \frac{1}{jq} - 2j\gamma G\eta_0 a^2 \frac{1}{1+a^2q^2} e^{jqvt}. \tag{53}$$

The X-ray diffraction signal at a momentum transfer $\vec{G} + \vec{q}$ is proportional to $|F|^2$. Retaining only the lowest order term in $Gu$, we find

$$|F|^2 = \frac{1}{q^2} + \frac{4\gamma G\eta_0 a^2}{q(1+a^2q^2)\cos{(qvt)}} = S_0 + \frac{1}{2}S_{osc}\cos{(qvt)}, \tag{54}$$

where $S_{osc}$ is the peak-to-peak oscillations amplitude and $S_0$ is the static signal. Showing their relation

$$\frac{S_{osc}}{S_0} = \frac{8\gamma G\eta_0 a^2 q}{1+a^2q^2}, \tag{55}$$

where we can finally obtain an estimate for the strain, $u$:

$$u = \eta_0 a = \frac{S_{osc}}{S_0}\frac{1+a^2q^2}{8\gamma Gaq} \tag{56}$$

Hence, by using Eq. (56), we can estimate the magnitude of acoustic strain displacement ($u$) from our experimental tr-XRD data. From the data of $\Delta\phi = -0.5°$, as shown in Fig. S8 and Table II, using the ratio of $S_{osc}/S_0$ for QL and QS modes, we obtain an acoustic displacement of $u_{QL} = 15.0$ pm and $u_{QS} = 12.6$ pm, representing the total displacement over the crystal volume defined by the carrier diffusion length ($\sim$70 nm) along the surface normal. These values are close to the calculated values ($u_{QL} = 25.9$ pm and $u_{QS} = 11.6$ pm) obtained from the elastic tensor in Sec. VII.

| $\Delta\phi$ <br> $q$ | -0.3° <br> 0.20 Å$^{-1}$ | | -0.5° <br> 0.33 Å$^{-1}$ | |
|---|---|---|---|---|
| | QL | QS | QL | QS |
| $\gamma$ | 0.64 | -0.49 | 0.64 | -0.49 |
| $S_{osc}/S_0$ | 0.063 | 0.044 | 0.085 | 0.052 |
| $u_{QL,QS}$ | 6.67 pm | 6.39 pm | 15.0 pm | 12.6 pm |
| $u_{QL}/u_{QS}$ | 1.04 | | 1.19 | |

TABLE II. The parameters used to calculate the acoustic displacement $u_{QL,QS}$ from Eq. (56)

However, we note the time delay chosen to extract the peak-to-peak ratio for the QL and QS amplitudes ($S_{osc}/S_0$) is arbitrary, exhibiting a time dependence that is shown in Fig. S9. Here, using fit results from a binary sinusoidal model (Eq. (2)) in the main text), we plot the time-dependent peak-to-peak ratio $S_{osc}/S_0$ for the QL and QS modes, respectively, in Fig. S9(a,b), and their relative ratio $A_{QL}/A_{QS}$ as a function of time delay in Fig. S9(c,d). Although our model assumes to take $S_{osc}/S_0$ at time delays far from $t = 0$, when the acoustic pulse is no longer near the surface boundary, the initial ratio of $A_{QL}/A_{QS}$ shows a values of $\sim 2$, which corresponds to a result of 2.2 obtained from our previous calculations in Sec. VI. However, for $t > 0$ this amplitude ratio drops to $\sim 1 - 0.5$ due to a difference in dephasing times between the QL and QS modes.

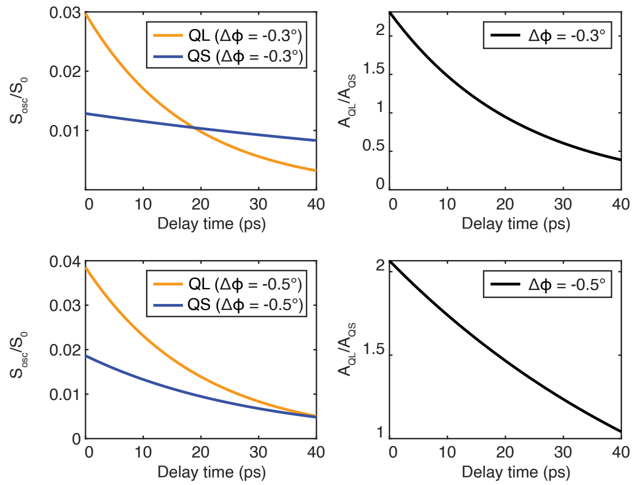


FIG. S9. Time-dependent amplitudes of the QL and QS modes and their relative ratio for (a,b) $\Delta\phi = -0.3°$ and (c,d) $-0.5°$.

## IX. MODELING THE ELECTRONIC STRUCTURE OF DYNAMICALLY STRAINED TAAS

In this section, we introduce a model calculation that describes how a dynamically strained crystal structure can produce changes in the electronic structure that are attributed to QL and QS lattice distortions. For temporal delays $t > 0$, an acoustic wave will propagate into the crystal at a sound velocity, $v$, introducing a structural distortions $u(z)$, as described by Eq. (52) due to the bipolar strain pulse, $du/dz$, given in Eq. (51) (assuming a symmetric shape). This is depicted schematically in Fig. S10(a), which shows a peak displacement of $z_0$ at a finite time delay $t_0 > 0$.

As a proof of principle, we model crystal structures with and without acoustic distortions using a $2\times2\times2$ supercell, as shown in Fig. S10(b). When modeling the effect of static, uniaxial strain from *ab initio*, lattice constraints orthogonal to the strain axis are relaxed to account for the Poisson effect, allowing for calculations to be performed on a single unit cell assuming periodic boundary conditions. In contrast, no such lattice deformation perpendicular to the strain axis occurs under dynamic strain, meaning a complete theoretical description of our experiment would require a large supercell having a length scale of a few tens of nanometers, equivalent to the wavelength of our acoustic modes. Practical limitations on computational time necessitates that we choose a smaller $2 \times 2 \times 2$ cell, which does introduce

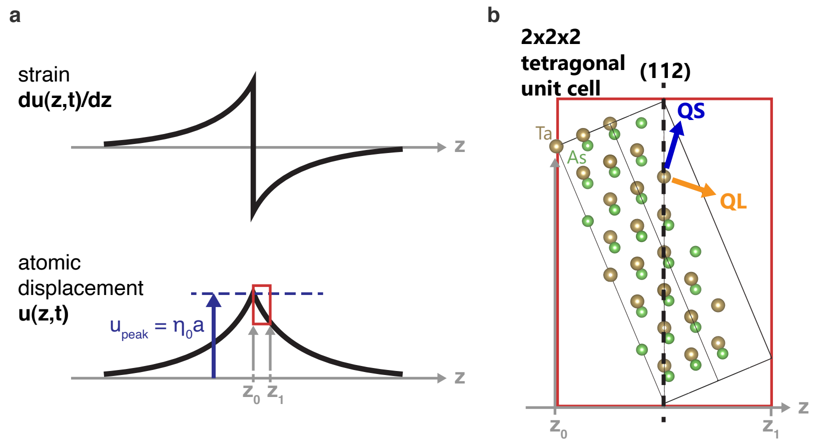


FIG. S10. (a) Profiles of optically-induced strain $(du/dz)$ and atomic displacement $(u)$ by acoustic phonons along the direction of the surface normal $(z)$. (b) Crystal structure in the $2 \times 2 \times 2$ tetragonal unit cell, where atomic positions are shifted by QL and QS distortions. The amount of distortions are set to be different depending on atomic positions relative to $z = z_0$.

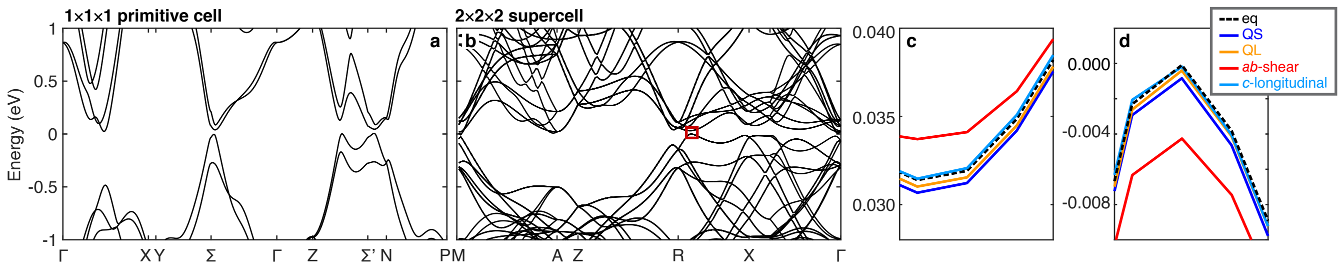


FIG. S11. Simulated electronic structures of TaAs from the crystal structures of (a) $1 \times 1 \times 1$ primitive cell and (b-d) $2 \times 2 \times 2$ cell. The electronic structures in equilibrium (black dashed line), after being shifted by 0.2 pm within the $2 \times 2 \times 2$ supercell for the QL (orange) and QS (blue) acoustic distortions, and for *ab*-plane shear (red) and *c*-axis longitudinal distortions (sky blue), are shown near the Weyl point.

an artificial periodicity to lattice distortions as compared to the experimental acoustic wavelength. Despite this computational simplification, we believe calculations using the experimentally inferred picometer displacements of the QL and QS modes, obtained from the peak-to-peak amplitude ratio measured at 10 ps from our tr-XRD experiments (Table II in Sec. VII), applied within the $2 \times 2 \times 2$ supercell can shed light on how QL and QS acoustic distortions can modify the electronic structure of TaAs, particulalry in vicinity of the Weyl nodes. To do so, we shifted atomic positions along the QL and QS directions, where the amount of distortion, $u(z, t)$, is relatively different for each atom depending on its distance from $z = z_0 = vt_0$ (the position for the largest QL and QS distortions) at a finite time delay $t_0 > 0$, as shown in Fig. S10(a).

Using these crystal structures, we performed first-principles calculations to simulate the electronic structure of TaAs under acoustic deformation. Here, we used the full-potential linearized augmented plane-wave (FP-LAPW) method of WIEN2K to carry out calculations on both the equilibrium and distorted crystal structures. Relativistic spin-orbit coupling effects were included using a $k$-point grid of 11×11×3 for each supercell and a 12×12×12 grid for primitive cell calculations.

Weyl points from the undistorted, equilibrium crystal structure are shown in Fig. S11(a-d), where small gaps are found at the Weyl nodes due to spin-orbit coupling [26, 27]. Here, electronic structure calculations from the primitive cell (Fig. S11(a)) show excellent agreement with previous calculations [26, 27]. When doubled, the electronic band structure from the undistorted $2 \times 2 \times 2$ supercell (Fig. S11(b)) is represented in a triclinic basis to directly compare with snapshots of the non-equilibrium structure following acoustic deformation (Fig. S11(c-d)). By shifting atomic positions by an amount estimated from our tr-XRD experiments, we find the low energy electronic structure in vicinity of the Weyl points to shift in energy with respect to equilibrium, indicating that both QL and QS distortions alter the low energy electronic structure of TaAs, while conserving the total number of Weyl nodes (Fig. S11(c,d)).

We similarly examined the effect of acoustic lattice displacement on the electronic structure under compressive and shear stress directed along more conventional crystal axes ((100), (010), (001)). Here, both a shear distortion in the *ab*-plane (*ab*-shear) and longitudinal distortion along the *c*-axis(*c*-longitudinal), result in changes to the electronic structure that are consistent with symmetry. Using the same sub-picometer distortion as estimated for the QS and QL modes, we find *c*-axis deformation does not alter the electronic structure with respect to equilibrium, while an in-plane shear distortions within the $2 \times 2 \times 2$ supercell creates a more noticeable change. Such a finding is consistent with the fact that the generation of LA phonons along (001) does not significantly alter the $4mm$ point group symmetry of TaAs, while shearing in the *ab*-plane can break mirror symmetries and change the energy and position of Weyl nodes reflected across these planes. These results suggest the most significant contribution in altering the low energy electronic structure of TaAs by QL and QS acoustic deformations can be attributed to shearing within the *ab*-plane.

[1] D. A. Reis and A. M. Lindenberg, in Light Scattering in Solids IX, edited by M. Cardona and R. Merlin (Springer-Verlag, Berlin, 2007), p. 371.
[2] C. P. Weber *et al.*, J. Appl. Phys. **122**, 223102 (2017).
[3] L. D. Landau and E. M. Lifshitz, *"Theory of Elasticity"*, Pergamon Press Oxford (1986).
[4] L. Liu, Z.-Q. Wang, C.-E. Hu, Y. Cheng, and G.-F. Ji, Solid State Commnu. **263**, 10 (2017).
[5] N. Sirica *et al.*, Phys. Rev. Lett. **122**, 197401 (2019).
[6] N. Sirica *et al.*, Nat. Mater. **21**, 62 (2022).

[7] P. Ruello and V. E. Gusev, Ultrasonics **56**, 21 (2015).
[8] M. Lejman, G. Vaudel, I. C. Infante, P. Gemeiner, V. E. Gusev, B. Dkhil, and P. Ruello, Nat. Commun. **5**, 4301 (2014).
[9] P. Giannozzi *et al.*, J. Phys. Condens. Matter **21**, 395502 (2009).
[10] D. R. Hamann, Phys. Rev. B **88**, 085117 (2013).
[11] S. Baroni, P. Giannozzi, and A. Testa, Phys. Rev. Lett. **58**, 1861 (1987).
[12] S. Baroni, S. de Gironcoli, A. Dal Corso, and P. Giannozzi, Rev. Mod. Phys. **73**, 515 (2001).
[13] X. Gonze, Phys. Rev. A **52**, 1096 (1995).
[14] H.-Y. Hao and H. J. Maris, Phys. Rev. Lett. **84**, 5556 (2000).
[15] C. L. Poyser, W. B. York, D. Srikanthreddy, B. A. Glavin, T. L. Linnik, R. P. Campion, A. V. Akimov, and A. J. Kent, Phys. Rev. Lett. **119**, 255502 (2017).
[16] C. Klieber, V. E. Gusev, T. Pezeril, and K. A. Nelson, Phys. Rev. Lett. **114**, 065701 (2015).
[17] B. A. Ruzicka, L. K. Werake, H. Samassekou, and H. Zhao, Appl. Phys. Lett. **97**, 262119 (2010).
[18] T. Shin, S. W. Teitelbaum, J. Wolfson, M. Kandyla, and K. A. Nelson, J. Chem. Phys. **143**, 194705 (2015).
[19] T. Pezeril, Opt. Laser Technol. **83**, 177 (2016).
[20] T. Pezeril, P. Ruello, S. Gougeon, N. Chigarev, D. Mounier, J.-M. Breteau, P. Picart, and V. Gusev, Phys. Rev. B **75**, 174307 (2007).
[21] B. A. Auld, *Acoustic fields and waves in solids*, Wiley, V. 1 (1973).
[22] T. Pezeril, V. Gusev, D. Mounier, N. Chigarev, P. Ruello, *Surface motion induced by laser action on opaque anisotropic crystals.* J. Phys. D: Appl. Phys. **38**, 1421 (2005).
[23] T. Pezeril PhD thesis. `https://tel.archives-ouvertes.fr/tel-00011291`.
[24] D. Chang, Y. Liu, F. Rao, F. Wang, Q. Sunac and Y. Jia, Phys. Chem. Chem. Phys. **18**, 14503 (2016).
[25] C.-L. Zhang *et al*, Nat. Commun. **7**, 10735 (2016).
[26] S.-M. Huang et al., Nat. Commun. **6**, 7373 (2015).
[27] H. Weng, C. Fang, Z. Fang, B. A. Bernevig, and X. Dai, Phys. Rev. X **5**, 011029 (2015).
